# Supplementary material for: Feature-aware Diversified Re-ranking with Disentangled Representations for Relevant Recommendation
Source: arXiv:2206.05020 source file (2022-06-10)
Supplement: Supplementary file 1 [file sec-appendix.tex]

\begin{appendices}

\section{Notations}
We list all the notations and the corresponding explanations in Table \ref{tab:notation} for a better understanding.

\begin{table}[]
\centering
\caption{Notations and Explanations}
\label{tab:notation}
\begin{tabular}{@{}cc@{}}
\toprule
\textbf{Notations} & \textbf{Explanation} \\ \midrule
       $u$            &    user                  \\
       $i$, $i^{'}$            &  item                 \\ 
       $i_t$            &  trigger item                 \\ 
       $\mathcal{I}, \mathcal{I}^{'}$  &  the set of item                 \\ 
       $\mathcal{R}$    &  the recommended set of item                 \\ 
       $\mathcal{F}_i$            &  the feature set of item $i$  \\
       $N$           & the number of item \\
       $F$           & the size of feature set \\
       $L$           & the length of recommended item\\
       $A$           & the number of latent aspect\\
       $d$           & the dimension of representation\\
       $\tau$           & the temperature parameter\\
       $\bm{e}_i \in \mathbb{R}^{d}$ & the representation of item $i$\\ 
       $\bm{F} \in \mathbb{R}^{F \times d}$ & the representation of feature set\\
       $\bm{q}^a \in \mathbb{R}^{d}$ & the $a$-th projected vector\\
       $\bm{P}^a \in \mathbb{R}^{F \times d}$ & the $a$-th projected matrix\\
       $\bm{v}^a \in \mathbb{R}^{d}$ & the representation of aspect $a$ \\
       $\widetilde{\bm{v}} \in \mathbb{R}^{d}$ & the average aspect representation\\
       $\bm{w}^R, \bm{w}^D \in \mathbb{R}^{A}$ &  the learnable coefficient vector\\
       $\bm{r} \in \mathbb{R}^{A}$ &  the accumulated relevance\\
       \bottomrule
\end{tabular}
\end{table}

\begin{table}[]
\centering
\caption{Parameter settings of all the compared algorithms in offline experiments. }
\label{tab:setting}
\begin{tabular}{@{}c|cc@{}}
\toprule
\textbf{Algorithm} & \multicolumn{2}{c}{\textbf{Parameter Settings}}                                                 \\ \midrule
\textbf{RR}        & \multicolumn{2}{c}{$\lambda$=3.5}                                                               \\ \midrule
\textbf{DPP}       & \multicolumn{2}{c}{\begin{tabular}[c]{@{}c@{}}$\lambda$=3.5\\ $\theta$=0.8\end{tabular}}                 \\ \midrule
\textbf{SSD}       & \multicolumn{2}{c}{\begin{tabular}[c]{@{}c@{}}$\lambda$=3.5\\ $\gamma$=1.5\end{tabular}}                 \\ \midrule
\textbf{MMR}       & \multicolumn{2}{c}{\begin{tabular}[c]{@{}c@{}}$\lambda$=3.5\\ $\theta$=0.7\end{tabular}}                 \\ \midrule
\multirow{2}{*}{\textbf{FDSB}} & \multicolumn{1}{c|}{\textbf{DAE}} & \begin{tabular}[c]{@{}c@{}}$d$=128\\$F$=15\\$A$=5\\ $\tau$=0.1\\ hidden \_size=[128, 64] \\batch\_size=8192\\learning\_rate=1e-3\\optimizer=Adam\end{tabular} \\ \cmidrule(l){2-3} 
                   & \multicolumn{1}{c|}{\textbf{Ranker}} & \begin{tabular}[c]{@{}c@{}}$\lambda$=3.5\\  $\theta$ =0.5\end{tabular} \\ \bottomrule
\end{tabular}
\end{table}

\section{Experiment Configuration}
The software environment of offline experiments is Linux, Python 3.8 and Pytorch 1.9.0. All the offline results of \ourmodel and other methods are produced by a machine with two GPUs~(\emph{NVIDIA TESLA T4}), one CPU~(\emph{Intel Xeon E5 2680}) and 128G memory.

We carefully tune the parameters for all the compared algorithms and report them in Table\ref{tab:setting}.

\end{appendices}
